# Supplementary material for: g2pM: A Neural Grapheme-to-Phoneme Conversion Package for Mandarin Chinese Based on a New Open Benchmark Dataset
Source: arXiv:2004.03136 source file (2020-09-17)
Supplement: Supplementary file 1 [file 9appendix.tex]

\section{Appendix}
\appendix
\section{100 most frequent polyphones and their frequencies}
的: 2.96\%, 中: 0.83\%, 大: 0.63\%, 和: 0.52\%, 了: 0.43\%, \\为: 0.41\%, 地: 0.40\%, 於: 0.38\%, 上: 0.37\%, 行: 0.35\%, \\作: 0.29\%, 分: 0.29\%, 同: 0.23\%, 子: 0.23\%, 可: 0.23\%, \\任: 0.22\%, 克: 0.21\%, 度: 0.19\%, 得: 0.19\%, 要: 0.18\%, \\教: 0.18\%, 会: 0.17\%, 合: 0.16\%, 区: 0.16\%, 化: 0.15\%, \\通: 0.15\%, 重: 0.14\%, 都: 0.14\%, 发: 0.13\%, 比: 0.13\%, \\王: 0.13\%, 省: 0.13\%, 相: 0.12\%, 正: 0.12\%, 系: 0.12\%, \\与: 0.12\%, 长: 0.11\%, 阿: 0.11\%, 女: 0.11\%, 量: 0.10\%, \\卡: 0.10\%, 曾: 0.09\%, 委: 0.09\%, 色: 0.09\%, 夫: 0.09\%, \\过: 0.08\%, 校: 0.08\%, 车: 0.08\%, 空: 0.08\%, 朝: 0.08\%, \\更: 0.08\%, 间: 0.08\%, 种: 0.08\%, 将: 0.07\%, 石: 0.07\%, \\少: 0.07\%, 曲: 0.07\%, 称: 0.07\%, 数: 0.07\%, 当: 0.07\%, \\解: 0.07\%, 只: 0.07\%, 属: 0.06\%, 角: 0.06\%, 片: 0.06\%, \\场: 0.06\%, 华: 0.06\%, 足: 0.06\%, 打: 0.05\%, 号: 0.05\%, \\居: 0.05\%, 语: 0.05\%, 服: 0.05\%, 广: 0.05\%, 令: 0.05\%, \\查: 0.05\%, 约: 0.05\%, 哈: 0.05\%, 好: 0.05\%, 勒: 0.05\%, \\率: 0.05\%, 供: 0.05\%, 单: 0.05\%, 伯: 0.05\%, 那: 0.04\%, \\参: 0.04\%, 还: 0.04\%, 落: 0.04\%, 模: 0.04\%, 塞: 0.04\%, \\万: 0.04\%, 氏: 0.04\%, 处: 0.04\%, 说: 0.04\%, 食: 0.04\%, \\奇: 0.04\%, 结: 0.04\%, 应: 0.04\%, 乐: 0.04\%, 传: 0.04\% \\
\label{appendix1}

\section{Polyphonic characters in the CPP dataset}
\tablefirsthead{\toprule \textbf{Polyphone} &\textbf{Total \# sents.} & \textbf{Pinyin (\# sents.)} \\ \midrule}

\tablehead{
\multicolumn{3}{c}
{{\bfseries  Continued from previous column}} \\
\toprule
\textbf{Polyphone}&\textbf{Total \# sents.}&\textbf{Pinyin (\# sents.)}\\ \midrule}

\tabletail{
\midrule \multicolumn{3}{c}{{Continued on next column}} \\ \midrule}
\tablelasttail{
\\\midrule
\multicolumn{3}{c}{{Concluded}} \\ \bottomrule}

\begin{supertabular}{lll}
    万 & 202 & wan4 (202), mo4 (0)\\ 
    上 & 201 & shang4 (201), shang3 (0)\\ 
    与 & 199 & yu3 (186), yu4 (13), yu2 (0)\\ 
    丧 & 189 & sang4 (131), sang1 (58)\\ 
    中 & 200 & zhong1 (197), zhong4 (3)\\ 
    为 & 193 & wei2 (177), wei4 (16)\\ 
    丽 & 202 & li4 (160), li2 (42)\\ 
    么 & 200 & me5 (200), ma2 (0), ma5 (0)\\ 
    乐 & 196 & yue4 (104), le4 (92)\\ 
    乘 & 188 & cheng2 (188), sheng4 (0)\\ 
    乙 & 199 & yi3 (199), zhe2 (0)\\ 
    了 & 202 & le5 (200), liao3 (2), liao4 (0)\\ 
    予 & 194 & yu3 (194), yu2 (0)\\ 
    亟 & 51 & ji2 (51), qi4 (0)\\ 
    亲 & 202 & qin1 (201), qing4 (1)\\ 
    亹 & 21 & wei3 (21), men2 (0)\\ 
    什 & 201 & shi2 (162), shen2 (39)\\ 
    仆 & 199 & pu2 (199), pu1 (0)\\ 
    仇 & 195 & chou2 (173), qiu2 (22)\\ 
    仔 & 163 & zai3 (120), zi3 (43), zi1 (0)\\ 
    仡 & 50 & ge1 (48), yi4 (2)\\ 
    令 & 196 & ling4 (196), ling2 (0), ling3 (0)\\ 
    价 & 195 & jia4 (195), jie5 (0)\\ 
    任 & 201 & ren4 (199), ren2 (2)\\ 
    会 & 202 & hui4 (202), kuai4 (0)\\ 
    传 & 201 & chuan2 (183), zhuan4 (18)\\ 
    伯 & 202 & bo2 (202), bai3 (0), ba4 (0)\\ 
    估 & 200 & gu1 (199), gu4 (1)\\ 
    伺 & 191 & si4 (167), ci4 (24)\\ 
    似 & 196 & si4 (196), shi4 (0)\\ 
    佃 & 150 & dian4 (150), tian2 (0)\\ 
    佚 & 202 & yi4 (202), die2 (0)\\ 
    佛 & 183 & fo2 (181), fu2 (2)\\ 
    作 & 202 & zuo4 (202), zuo1 (0)\\ 
    佣 & 198 & yong1 (187), yong4 (11)\\ 
    侗 & 200 & dong4 (157), tong2 (43)\\ 
    供 & 197 & gong1 (175), gong4 (22)\\ 
    侧 & 202 & ce4 (202), zhai1 (0)\\ 
    便 & 200 & bian4 (197), pian2 (3)\\ 
    俊 & 202 & jun4 (202), zun4 (0)\\ 
    俞 & 201 & yu2 (201), shu4 (0)\\ 
    俟 & 149 & si4 (125), qi2 (24)\\ 
    倒 & 191 & dao3 (134), dao4 (57)\\ 
    倘 & 148 & tang3 (148), chang2 (0)\\ 
    假 & 200 & jia3 (143), jia4 (57), gei1 (0)\\ 
    偈 & 51 & ji4 (51), jie2 (0)\\ 
    偻 & 11 & lu:3 (6), lou2 (5)\\ 
    傀 & 200 & kui3 (200), gui1 (0)\\ 
    僮 & 96 & tong2 (55), zhuang4 (41)\\ 
    儿 & 202 & er2 (197), r5 (5), ren2 (0)\\ 
    克 & 202 & ke4 (202), kei1 (0)\\ 
    免 & 202 & mian3 (202), wen4 (0)\\ 
    兴 & 199 & xing1 (181), xing4 (18)\\ 
    冠 & 198 & guan4 (163), guan1 (35)\\ 
    冯 & 202 & feng2 (202), ping2 (0)\\ 
    冲 & 199 & chong1 (198), chong4 (1)\\ 
    凉 & 200 & liang2 (200), liang4 (0)\\ 
    几 & 201 & ji3 (160), ji1 (41)\\ 
    凹 & 200 & ao1 (196), wa1 (4)\\ 
    分 & 171 & fen1 (170), fen4 (1)\\ 
    切 & 123 & qie4 (66), qie1 (57)\\ 
    划 & 195 & hua4 (191), hua2 (4)\\ 
    创 & 200 & chuang4 (194), chuang1 (6)\\ 
    刨 & 48 & bao4 (25), pao2 (23)\\ 
    别 & 202 & bie2 (202), bie4 (0)\\ 
    刷 & 199 & shua1 (199), shua4 (0)\\ 
    刹 & 121 & cha4 (92), sha1 (29)\\ 
    刺 & 202 & ci4 (202), ci1 (0)\\ 
    削 & 199 & xue1 (169), xiao1 (30)\\ 
    剌 & 201 & la4 (201), la2 (0)\\ 
    剡 & 44 & shan4 (43), yan3 (1)\\ 
    剥 & 199 & bo1 (175), bao1 (24)\\ 
    剿 & 200 & jiao3 (200), chao1 (0)\\ 
    劈 & 201 & pi1 (196), pi3 (5)\\ 
    劲 & 201 & jing4 (115), jin4 (86)\\ 
    勒 & 202 & le4 (201), lei1 (1)\\ 
    勾 & 202 & gou1 (198), gou4 (4)\\ 
    化 & 202 & hua4 (202), hua1 (0)\\ 
    匮 & 176 & kui4 (175), gui4 (1)\\ 
    匹 & 201 & pi3 (201), pi1 (0)\\ 
    区 & 202 & qu1 (202), ou1 (0)\\ 
    匾 & 201 & bian3 (201), pian2 (0)\\ 
    华 & 200 & hua2 (200), hua4 (0), hua1 (0)\\ 
    卒 & 199 & zu2 (198), cu4 (1)\\ 
    单 & 197 & dan1 (196), shan4 (1)\\ 
    卜 & 189 & bu3 (170), bo5 (19)\\ 
    占 & 201 & zhan4 (197), zhan1 (4)\\ 
    卡 & 202 & ka3 (201), qia3 (1)\\ 
    卷 & 199 & juan4 (133), juan3 (66)\\ 
    厂 & 202 & chang3 (202), han3 (0)\\ 
    压 & 202 & ya1 (202), ya4 (0)\\ 
    厕 & 196 & ce4 (196), si4 (0)\\ 
    厦 & 200 & sha4 (103), xia4 (97)\\ 
    参 & 202 & can1 (199), shen1 (3)\\ 
    叉 & 181 & cha1 (181), cha3 (0), cha2 (0)\\ 
    发 & 201 & fa1 (198), fa4 (3)\\ 
    句 & 197 & ju4 (140), gou1 (57)\\ 
    叨 & 19 & dao1 (19), tao1 (0)\\ 
    只 & 191 & zhi3 (173), zhi1 (18)\\ 
    召 & 193 & zhao4 (193), shao4 (0)\\ 
    可 & 202 & ke3 (201), ke4 (1)\\ 
    叶 & 202 & ye4 (202), xie2 (0)\\ 
    号 & 201 & hao4 (201), hao2 (0)\\ 
    吁 & 199 & yu4 (199), xu1 (0)\\ 
    合 & 202 & he2 (202), ge3 (0)\\ 
    同 & 201 & tong2 (200), tong4 (1)\\ 
    吐 & 198 & tu3 (173), tu4 (25)\\ 
    吒 & 100 & zha1 (58), zha4 (42)\\ 
    吓 & 200 & xia4 (128), he4 (72)\\ 
    吗 & 201 & ma5 (170), ma3 (31)\\ 
    否 & 202 & fou3 (202), pi3 (0)\\ 
    吧 & 200 & ba1 (123), ba5 (77), bia1 (0)\\ 
    听 & 194 & ting1 (194), yin3 (0), ting4 (0)\\ 
    吱 & 25 & zhi1 (25), zi1 (0)\\ 
    呐 & 151 & na4 (147), na5 (4)\\ 
    呗 & 21 & bai4 (13), bei5 (8)\\ 
    呛 & 18 & qiang4 (16), qiang1 (2)\\ 
    呢 & 199 & ne5 (175), ni2 (24)\\ 
    呵 & 99 & he1 (95), a1 (4)\\ 
    咋 & 15 & za3 (7), ze2 (5), zha4 (3)\\ 
    \multirow{2}{*}{和} & \multirow{2}{*}{201} & \multirow{2}{*}{he2 (201), huo4 (0), hu2 (0),}\\
    {}&{}&\multirow{2}{*}{he4 (0), huo2 (0)} \\
    {}&{}&{}\\
    咥 & 19 & die2 (19), xi4 (0)\\ 
    咧 & 11 & lie1 (6), lie3 (5), lie5 (0)\\ 
    咯 & 146 & luo4 (80), ge1 (63), lo5 (3)\\ 
    咱 & 81 & zan2 (81), za2 (0)\\ 
    咳 & 195 & ke2 (195), hai1 (0)\\ 
    咽 & 200 & yan1 (155), yan4 (35), ye4 (10)\\ 
    哄 & 48 & hong1 (20), hong3 (20), hong4 (8)\\ 
    哇 & 180 & wa1 (180), wa5 (0)\\ 
    哈 & 202 & ha1 (201), ha3 (1)\\ 
    哏 & 51 & gen2 (51), hen3 (0)\\ 
    哑 & 202 & ya3 (202), ya1 (0)\\ 
    哗 & 201 & hua2 (196), hua1 (5)\\ 
    哟 & 32 & yo5 (27), yo1 (5)\\ 
    哦 & 43 & o4 (34), o5 (8), o2 (1), e2 (0)\\ 
    哩 & 106 & li3 (102), li5 (4)\\ 
    哪 & 187 & na3 (184), na5 (3), nei3 (0)\\ 
    哺 & 202 & bu3 (202), bu1 (0), bu4 (0)\\ 
    唉 & 12 & ai4 (10), ai1 (2)\\ 
    唠 & 12 & lao2 (10), lao4 (2)\\ 
    唯 & 202 & wei2 (202), wei3 (0)\\ 
    唷 & 7 & yo1 (7), yo5 (0)\\ 
    啊 & 186 & a5 (155), a4 (26), a1 (5), a2 (0), a3 (0)\\ 
    啦 & 195 & la1 (143), la5 (52)\\ 
    啰 & 49 & luo1 (47), luo5 (2)\\ 
    喂 & 201 & wei4 (200), wei2 (1)\\ 
    喇 & 201 & la3 (200), la1 (1)\\ 
    喔 & 11 & wo5 (11), o1 (0)\\ 
    喝 & 192 & he1 (176), he4 (16)\\ 
    喳 & 7 & zha1 (5), cha1 (2)\\ 
    喷 & 202 & pen1 (202), pen4 (0)\\ 
    嗯 & 17 & en4 (11), en1 (6), en5 (0)\\ 
    嘌 & 102 & piao4 (102), piao1 (0)\\ 
    嘲 & 200 & chao2 (200), zhao1 (0)\\ 
    噌 & 12 & ceng1 (12), cheng1 (0)\\ 
    嚓 & 20 & ca1 (11), cha1 (9)\\ 
    囤 & 86 & tun2 (83), dun4 (3)\\ 
    囱 & 193 & cong1 (193), chuang1 (0)\\ 
    圈 & 199 & quan1 (194), juan4 (5), juan1 (0)\\ 
    圜 & 95 & huan2 (57), yuan2 (38)\\ 
    圩 & 194 & wei2 (183), xu1 (11)\\ 
    地 & 201 & di4 (185), de5 (16)\\ 
    场 & 202 & chang3 (202), chang2 (0)\\ 
    坊 & 189 & fang1 (149), fang2 (40)\\ 
    坻 & 101 & di3 (101), chi2 (0)\\ 
    垛 & 188 & duo3 (159), duo4 (29)\\ 
    埋 & 200 & mai2 (200), man2 (0)\\ 
    埏 & 22 & yan2 (22), shan1 (0)\\ 
    埔 & 198 & pu3 (194), bu4 (4)\\ 
    堡 & 198 & bao3 (198), pu4 (0)\\ 
    塞 & 197 & sai4 (191), se4 (4), sai1 (2)\\ 
    处 & 170 & chu4 (121), chu3 (49)\\ 
    大 & 201 & da4 (201), dai4 (0)\\ 
    夫 & 202 & fu1 (202), fu2 (0)\\ 
    夯 & 198 & hang1 (195), ben4 (3)\\ 
    头 & 193 & tou2 (191), tou5 (2)\\ 
    夹 & 202 & jia1 (190), jia2 (12), jia4 (0)\\ 
    奄 & 148 & yan3 (148), yan1 (0)\\ 
    奇 & 200 & qi2 (198), ji1 (2)\\ 
    奔 & 183 & ben1 (112), ben4 (71)\\ 
    奘 & 150 & zang4 (150), zhuang3 (0)\\ 
    女 & 202 & nu:3 (202), ru3 (0)\\ 
    好 & 201 & hao3 (178), hao4 (23)\\ 
    妻 & 202 & qi1 (202), qi4 (0)\\ 
    委 & 201 & wei3 (201), wei1 (0)\\ 
    姥 & 185 & lao3 (111), mu3 (74)\\ 
    娜 & 202 & na4 (202), nuo2 (0)\\ 
    娩 & 151 & mian3 (151), wan3 (0)\\ 
    媛 & 189 & yuan2 (166), yuan4 (23)\\ 
    嬛 & 22 & huan2 (22), xuan1 (0), qiong2 (0)\\ 
    子 & 190 & zi3 (149), zi5 (41)\\ 
    孱 & 42 & chan2 (42), can4 (0)\\ 
    宁 & 198 & ning2 (198), ning4 (0)\\ 
    宿 & 200 & su4 (169), xiu4 (30), xiu3 (1)\\ 
    将 & 195 & jiang1 (162), jiang4 (33), qiang1 (0)\\ 
    少 & 201 & shao3 (134), shao4 (67)\\ 
    尺 & 202 & chi3 (202), che3 (0)\\ 
    尽 & 197 & jin3 (118), jin4 (79)\\ 
    尾 & 202 & wei3 (202), yi3 (0)\\ 
    尿 & 202 & niao4 (202), sui1 (0)\\ 
    居 & 202 & ju1 (202), ji1 (0)\\ 
    屏 & 202 & ping2 (201), bing3 (1), bing1 (0)\\ 
    属 & 202 & shu3 (202), zhu3 (0)\\ 
    屯 & 202 & tun2 (202), zhun1 (0)\\ 
    岂 & 195 & qi3 (195), kai3 (0)\\ 
    峇 & 101 & ba1 (100), ke4 (1), ke1 (0)\\ 
    峒 & 87 & tong2 (68), dong4 (19)\\ 
    崭 & 200 & zhan3 (200), chan2 (0)\\ 
    崴 & 22 & wei1 (20), wai3 (2)\\ 
    嵌 & 200 & qian4 (199), kan3 (1)\\ 
    巂 & 52 & xi1 (52), gui1 (0)\\ 
    差 & 192 & cha1 (144), cha4 (37), chai1 (11)\\ 
    帖 & 192 & tie3 (190), tie1 (2), tie4 (0)\\ 
    幢 & 191 & zhuang4 (151), chuang2 (40)\\ 
    干 & 187 & gan1 (98), gan4 (89)\\ 
    广 & 202 & guang3 (202), yan3 (0)\\ 
    庑 & 200 & wu3 (200), wu2 (0)\\ 
    应 & 200 & ying4 (164), ying1 (36)\\ 
    底 & 200 & di3 (200), de5 (0)\\ 
    度 & 202 & du4 (202), duo2 (0)\\ 
    廑 & 19 & jin3 (19), qin2 (0)\\ 
    弄 & 197 & nong4 (141), long4 (56)\\ 
    弟 & 202 & di4 (202), ti4 (0)\\ 
    弹 & 199 & dan4 (157), tan2 (42)\\ 
    强 & 202 & qiang2 (197), qiang3 (5), jiang4 (0)\\ 
    当 & 197 & dang1 (193), dang4 (4)\\ 
    待 & 193 & dai4 (193), dai1 (0)\\ 
    得 & 197 & de2 (169), de5 (28), dei3 (0)\\ 
    徼 & 17 & jiao4 (12), jiao3 (5)\\ 
    忒 & 202 & te4 (202), tei1 (0)\\ 
    恁 & 10 & nen4 (8), nin2 (2)\\ 
    恶 & 193 & e4 (175), wu4 (11), e3 (7)\\ 
    悄 & 199 & qiao1 (167), qiao3 (32)\\ 
    悝 & 46 & kui1 (46), li3 (0)\\ 
    戌 & 199 & xu1 (199), qu5 (0)\\ 
    扁 & 202 & bian3 (202), pian1 (0)\\ 
    扇 & 201 & shan4 (196), shan1 (5)\\ 
    扎 & 202 & zha1 (200), zha2 (1), za1 (1)\\ 
    扒 & 134 & pa2 (79), ba1 (55)\\ 
    打 & 200 & da3 (200), da2 (0)\\ 
    扛 & 100 & kang2 (88), gang1 (12)\\ 
    扫 & 202 & sao3 (200), sao4 (2)\\ 
    扳 & 198 & ban1 (198), pan1 (0)\\ 
    把 & 201 & ba3 (201), ba4 (0)\\ 
    折 & 200 & zhe2 (200), she2 (0), zhe1 (0)\\ 
    抡 & 28 & lun2 (22), lun1 (6)\\ 
    抢 & 202 & qiang3 (202), qiang1 (0)\\ 
    抹 & 156 & mo3 (148), mo4 (4), ma1 (4)\\ 
    拂 & 201 & fu2 (201), bi4 (0)\\ 
    担 & 193 & dan1 (190), dan4 (3)\\ 
    拓 & 200 & tuo4 (195), ta4 (5)\\ 
    拗 & 40 & niu4 (35), ao4 (5)\\ 
    拚 & 10 & pin1 (10), pan4 (0)\\ 
    拧 & 42 & ning3 (35), ning2 (7), ning4 (0)\\ 
    \multirow{2}{*}{拽} & \multirow{2}{*}{91} & \multirow{2}{*}{zhuai4 (91), ye4 (0),}\\ 
    {} & {} & \multirow{2}{*}{zhuai3 (0), zhuai1 (0)} \\
    {}& {}& {} \\
    拾 & 199 & shi2 (199), she4 (0)\\ 
    挑 & 195 & tiao3 (152), tiao1 (43)\\ 
    挝 & 200 & wo1 (199), zhua1 (1)\\ 
    挟 & 173 & xie2 (172), jia1 (1)\\ 
    挡 & 197 & dang3 (197), dang4 (0)\\ 
    挣 & 201 & zheng1 (122), zheng4 (79)\\ 
    挨 & 198 & ai1 (111), ai2 (87)\\ 
    捋 & 12 & lu:3 (7), luo1 (5)\\ 
    据 & 202 & ju4 (202), ju1 (0)\\ 
    掖 & 196 & ye4 (196), ye1 (0)\\ 
    掺 & 200 & chan1 (200), shan3 (0)\\ 
    揣 & 98 & chuai3 (57), chuai1 (41)\\ 
    搁 & 200 & ge1 (200), ge2 (0)\\ 
    搂 & 12 & lou3 (12), lou1 (0)\\ 
    摸 & 202 & mo1 (202), mo2 (0)\\ 
    撇 & 94 & pie3 (53), pie1 (41)\\ 
    撒 & 199 & sa1 (190), sa3 (9)\\ 
    撩 & 14 & liao2 (9), liao1 (5)\\ 
    撮 & 150 & cuo1 (140), zuo3 (10)\\ 
    擂 & 190 & lei4 (116), lei2 (74)\\ 
    操 & 202 & cao1 (202), cao4 (0)\\ 
    攒 & 196 & cuan2 (133), zan3 (63)\\ 
    教 & 202 & jiao4 (200), jiao1 (2)\\ 
    敛 & 200 & lian3 (200), lian4 (0)\\ 
    散 & 193 & san4 (159), san3 (34)\\ 
    数 & 199 & shu4 (195), shu3 (2), shuo4 (2)\\ 
    斗 & 191 & dou4 (175), dou3 (16)\\ 
    旄 & 21 & mao2 (21), mao4 (0)\\ 
    旋 & 201 & xuan2 (198), xuan4 (3)\\ 
    晃 & 92 & huang4 (91), huang3 (1)\\ 
    晕 & 199 & yun1 (126), yun4 (73)\\ 
    晟 & 202 & sheng4 (202), cheng2 (0)\\ 
    曲 & 192 & qu3 (159), qu1 (33)\\ 
    更 & 202 & geng4 (146), geng1 (56)\\ 
    曾 & 196 & ceng2 (180), zeng1 (16)\\ 
    服 & 201 & fu2 (201), fu4 (0)\\ 
    朝 & 201 & chao2 (201), zhao1 (0)\\ 
    朮 & 6 & shu4 (4), zhu2 (2)\\ 
    术 & 202 & shu4 (202), zhu2 (0)\\ 
    朴 & 193 & pu3 (96), piao2 (96), po4 (1)\\ 
    杆 & 188 & gan1 (135), gan3 (53)\\ 
    杈 & 26 & cha4 (24), cha1 (2)\\ 
    杓 & 136 & shao2 (132), biao1 (4)\\ 
    杠 & 201 & gang4 (201), gang1 (0)\\ 
    杷 & 101 & pa2 (101), ba4 (0)\\ 
    杻 & 10 & niu3 (10), chou3 (0)\\ 
    板 & 202 & ban3 (202), pan4 (0)\\ 
    枸 & 50 & gou3 (47), ju3 (3), gou1 (0)\\ 
    柏 & 190 & bo2 (146), bai3 (44), bo4 (0)\\ 
    柜 & 199 & gui4 (199), ju3 (0)\\ 
    查 & 157 & cha2 (157), zha1 (0)\\ 
    校 & 200 & xiao4 (195), jiao4 (5)\\ 
    桁 & 199 & heng2 (199), hang2 (0)\\ 
    桄 & 7 & guang1 (7), guang4 (0)\\ 
    桔 & 201 & ju2 (133), jie2 (68)\\ 
    档 & 198 & dang4 (198), dang3 (0)\\ 
    棹 & 31 & zhao4 (31), zhuo1 (0)\\ 
    椎 & 200 & zhui1 (197), chui2 (3)\\ 
    楂 & 102 & zha1 (102), cha2 (0)\\ 
    楞 & 202 & leng2 (202), leng4 (0)\\ 
    楷 & 202 & kai3 (201), jie1 (1)\\ 
    槛 & 194 & kan3 (174), jian4 (20)\\ 
    樘 & 21 & cheng3 (15), tang2 (6)\\ 
    模 & 198 & mo2 (195), mu2 (3)\\ 
    横 & 199 & heng2 (193), heng4 (6)\\ 
    正 & 202 & zheng4 (198), zheng1 (4)\\ 
    歪 & 202 & wai1 (202), wai3 (0)\\ 
    殷 & 202 & yin1 (202), yin3 (0), yan1 (0)\\ 
    毂 & 51 & gu3 (51), gu1 (0)\\ 
    比 & 202 & bi3 (202), bi1 (0), bi4 (0)\\ 
    氏 & 202 & shi4 (201), zhi1 (1)\\ 
    氐 & 97 & di1 (97), di3 (0)\\ 
    氓 & 151 & mang2 (121), meng2 (30)\\ 
    汗 & 123 & han4 (67), han2 (56)\\ 
    汞 & 201 & gong3 (201), hong4 (0)\\ 
    汤 & 202 & tang1 (202), shang1 (0)\\ 
    沈 & 202 & shen3 (202), chen2 (0)\\ 
    沉 & 202 & chen2 (202), chen1 (0)\\ 
    沓 & 51 & ta4 (51), da2 (0)\\ 
    没 & 201 & mei2 (185), mo4 (16)\\ 
    沤 & 11 & ou1 (7), ou4 (4)\\ 
    泊 & 187 & po1 (100), bo2 (87)\\ 
    泡 & 179 & pao4 (162), pao1 (17)\\ 
    泥 & 201 & ni2 (199), ni4 (2)\\ 
    泷 & 102 & long2 (88), shuang1 (14)\\ 
    浅 & 194 & qian3 (194), jian1 (0)\\ 
    浆 & 202 & jiang1 (201), jiang4 (1)\\ 
    济 & 191 & ji4 (178), ji3 (13)\\ 
    浜 & 10 & bin1 (10), bang1 (0)\\ 
    涌 & 198 & yong3 (174), chong1 (24)\\ 
    涡 & 184 & wo1 (175), guo1 (9)\\ 
    涨 & 202 & zhang3 (199), zhang4 (3)\\ 
    淋 & 201 & lin2 (198), lin4 (3)\\ 
    混 & 200 & hun4 (200), hun2 (0)\\ 
    渐 & 202 & jian4 (202), jian1 (0)\\ 
    渠 & 202 & qu2 (202), ju4 (0)\\ 
    湮 & 152 & yan1 (152), yin1 (0)\\ 
    溇 & 10 & lou2 (10), lu:3 (0)\\ 
    溺 & 199 & ni4 (199), niao4 (0)\\ 
    漂 & 201 & piao1 (137), piao4 (48), piao3 (16)\\ 
    澄 & 192 & cheng2 (190), deng4 (2)\\ 
    澹 & 98 & dan4 (93), tan2 (5)\\ 
    濯 & 51 & zhuo2 (51), zhao4 (0)\\ 
    瀑 & 200 & pu4 (200), bao4 (0)\\ 
    炅 & 97 & jiong3 (97), gui4 (0)\\ 
    炔 & 199 & que1 (199), gui4 (0)\\ 
    炮 & 200 & pao4 (200), pao2 (0), bao1 (0)\\ 
    炸 & 202 & zha4 (191), zha2 (11)\\ 
    焌 & 12 & jun4 (12), qu1 (0)\\ 
    煞 & 87 & sha4 (85), sha1 (2)\\ 
    熜 & 31 & cong1 (31), zong3 (0)\\ 
    熨 & 50 & yun4 (49), yu4 (1)\\ 
    熬 & 195 & ao2 (194), ao1 (1)\\ 
    燎 & 99 & liao2 (98), liao3 (1)\\ 
    燕 & 155 & yan1 (79), yan4 (76)\\ 
    爪 & 127 & zhao3 (116), zhua3 (11)\\ 
    片 & 92 & pian4 (92), pian1 (0)\\ 
    牟 & 112 & mu4 (66), mou2 (46)\\ 
    率 & 201 & lu:4 (124), shuai4 (77)\\ 
    王 & 202 & wang2 (202), wang4 (0)\\ 
    玟 & 32 & wen2 (32), min2 (0)\\ 
    琢 & 149 & zhuo2 (144), zuo2 (5)\\ 
    瑱 & 52 & tian4 (52), zhen4 (0)\\ 
    甚 & 202 & shen4 (201), shen2 (1)\\ 
    甬 & 201 & yong3 (201), tong3 (0)\\ 
    町 & 198 & ting3 (196), ding1 (2)\\ 
    畜 & 200 & chu4 (118), xu4 (82)\\ 
    番 & 186 & fan1 (160), pan1 (26)\\ 
    畲 & 201 & she1 (201), yu2 (0)\\ 
    疟 & 199 & nu:e4 (199), yao4 (0)\\ 
    疸 & 52 & dan3 (52), da5 (0)\\ 
    症 & 202 & zheng4 (202), zheng1 (0)\\ 
    的 & 202 & de5 (202), di4 (0), di2 (0), di1 (0)\\ 
    监 & 197 & jian1 (185), jian4 (12)\\ 
    盖 & 201 & gai4 (199), ge3 (2)\\ 
    盛 & 202 & sheng4 (200), cheng2 (2)\\ 
    相 & 194 & xiang1 (161), xiang4 (33)\\ 
    省 & 200 & sheng3 (197), xing3 (3)\\ 
    看 & 201 & kan4 (197), kan1 (4)\\ 
    眯 & 10 & mi1 (10), mi2 (0)\\ 
    \multirow{2}{*}{着} & \multirow{2}{*}{195} & \multirow{2}{*}{zhe5 (190), zhuo2 (3),}\\ 
    \multirow{2}{*}{} & \multirow{2}{*}{} & \multirow{2}{*}{zhao2 (2), zhao1 (0)}\\
    {} & {} & {} \\
    矫 & 198 & jiao3 (197), jiao2 (1)\\ 
    石 & 202 & shi2 (201), dan4 (1)\\ 
    硐 & 42 & dong4 (42), tong2 (0)\\ 
    碌 & 146 & lu4 (146), liu4 (0)\\ 
    磕 & 52 & ke1 (52), ke4 (0)\\ 
    磨 & 176 & mo2 (143), mo4 (33)\\ 
    祭 & 198 & ji4 (198), zhai4 (0)\\ 
    禁 & 201 & jin4 (199), jin1 (2)\\ 
    禅 & 187 & chan2 (187), shan4 (0)\\ 
    禺 & 202 & yu2 (202), ou3 (0), yu4 (0)\\ 
    离 & 202 & li2 (202), chi1 (0)\\ 
    种 & 196 & zhong3 (195), zhong4 (1)\\ 
    秘 & 202 & mi4 (179), bi4 (23)\\ 
    秤 & 89 & cheng4 (89), cheng1 (0)\\ 
    称 & 201 & cheng1 (195), chen4 (6), cheng4 (0)\\ 
    稍 & 200 & shao1 (200), shao4 (0)\\ 
    稽 & 202 & ji1 (202), qi3 (0)\\ 
    空 & 200 & kong1 (198), kong4 (2)\\ 
    窨 & 23 & yin4 (23), xun1 (0)\\ 
    竺 & 200 & zhu2 (200), du3 (0)\\ 
    笼 & 198 & long2 (193), long3 (5)\\ 
    答 & 197 & da2 (177), da1 (20)\\ 
    簸 & 49 & bo3 (34), bo4 (15)\\ 
    粘 & 185 & nian2 (181), zhan1 (4)\\ 
    粥 & 200 & zhou1 (196), yu4 (4)\\ 
    糊 & 54 & hu2 (41), hu4 (13)\\ 
    糜 & 146 & mi2 (144), mei2 (2)\\ 
    系 & 200 & xi4 (199), ji4 (1)\\ 
    累 & 187 & lei3 (138), lei2 (26), lei4 (23)\\ 
    絜 & 19 & jie2 (19), xie2 (0)\\ 
    繇 & 7 & yao2 (7), zhou4 (0), you2 (0)\\ 
    纤 & 201 & xian1 (199), qian4 (2)\\ 
    纥 & 178 & he2 (178), ge1 (0)\\ 
    约 & 202 & yue1 (202), yao1 (0)\\ 
    纪 & 202 & ji4 (200), ji3 (2)\\ 
    结 & 202 & jie2 (202), jie1 (0)\\ 
    给 & 198 & gei3 (186), ji3 (12)\\ 
    络 & 201 & luo4 (201), lao4 (0)\\ 
    绦 & 41 & tao1 (41), di2 (0)\\ 
    绰 & 202 & chuo4 (202), chao1 (0)\\ 
    绷 & 101 & beng1 (99), beng3 (2)\\ 
    综 & 202 & zong1 (202), zeng4 (0)\\ 
    缀 & 202 & zhui4 (202), chuo4 (0)\\ 
    缉 & 202 & ji1 (202), qi1 (0)\\ 
    缊 & 16 & yun4 (16), yun1 (0)\\ 
    缝 & 193 & feng4 (132), feng2 (61)\\ 
    \multirow{2}{*}{缪} & \multirow{2}{*}{187} &\multirow{2}{*}{miu4 (150), miao4 (34), mou2 (2), } \\ 
    \multirow{2}{*}{} & \multirow{2}{*}{} & \multirow{2}{*}{mu4 (1), liao3 (0)}\\
    {}& {}& {} \\
    缯 & 51 & zeng1 (51), zeng4 (0)\\ 
    罢 & 200 & ba4 (200), ba5 (0)\\ 
    翘 & 196 & qiao4 (163), qiao2 (33)\\ 
    翟 & 197 & zhai2 (188), di2 (9)\\ 
    耙 & 51 & pa2 (51), ba4 (0)\\ 
    耶 & 200 & ye1 (199), ye2 (1), ye5 (0)\\ 
    肖 & 196 & xiao1 (148), xiao4 (48)\\ 
    肚 & 193 & du4 (161), du3 (32)\\ 
    背 & 198 & bei4 (195), bei1 (3)\\ 
    胖 & 201 & pang4 (199), pan2 (2)\\ 
    脉 & 202 & mai4 (202), mo4 (0)\\ 
    脏 & 201 & zang4 (186), zang1 (15)\\ 
    脚 & 201 & jiao3 (201), jue2 (0)\\ 
    脯 & 49 & fu3 (46), pu2 (3)\\ 
    腊 & 202 & la4 (202), xi1 (0)\\ 
    \multirow{2}{*}{膀} & \multirow{2}{*}{201} &\multirow{2}{*}{bang3 (138), pang2 (63),} \\ 
    \multirow{2}{*}{} & \multirow{2}{*}{} & \multirow{2}{*}{pang1 (0), bang4 (0)}\\
    {}& {}& {} \\
    膏 & 202 & gao1 (202), gao4 (0)\\ 
    臊 & 20 & sao4 (16), sao1 (4)\\ 
    臭 & 202 & chou4 (187), xiu4 (15)\\ 
    舍 & 201 & she4 (184), she3 (17)\\ 
    般 & 202 & ban1 (201), pan2 (1)\\ 
    艮 & 202 & gen4 (201), gen3 (1)\\ 
    色 & 202 & se4 (202), shai3 (0)\\ 
    艾 & 202 & ai4 (202), yi4 (0)\\ 
    节 & 202 & jie2 (202), jie1 (0)\\ 
    芍 & 11 & que4 (11), shao2 (0)\\ 
    芥 & 202 & jie4 (202), gai4 (0)\\ 
    芯 & 202 & xin1 (202), xin4 (0)\\ 
    芸 & 202 & yun2 (202), yi4 (0)\\ 
    芾 & 62 & fu2 (54), fei4 (8)\\ 
    苔 & 202 & tai2 (201), tai1 (1)\\ 
    苕 & 81 & tiao2 (72), shao2 (9)\\ 
    茄 & 198 & qie2 (187), jia1 (11)\\ 
    茆 & 32 & mao2 (32), mao3 (0)\\ 
    茜 & 196 & qian4 (130), xi1 (66)\\ 
    草 & 202 & cao3 (202), cao4 (0)\\ 
    荑 & 11 & ti2 (11), yi2 (0)\\ 
    荠 & 37 & qi2 (33), ji4 (4)\\ 
    荡 & 201 & dang4 (201), tang4 (0)\\ 
    荷 & 196 & he2 (179), he4 (17)\\ 
    莎 & 200 & sha1 (159), suo1 (41)\\ 
    莘 & 127 & shen1 (72), xin1 (55)\\ 
    \multirow{2}{*}{莞} & \multirow{2}{*}{194} &\multirow{2}{*}{guan3 (191), wan3 (2)} \\ 
    \multirow{2}{*}{} & \multirow{2}{*}{} & \multirow{2}{*}{guan1 (1}\\
    {} & {} & {} \\
    莳 & 12 & shi4 (9), shi2 (3)\\ 
    菌 & 195 & jun1 (195), jun4 (0)\\ 
    菲 & 202 & fei1 (202), fei3 (0)\\ 
    菸 & 30 & yan1 (30), yu1 (0)\\ 
    落 & 201 & luo4 (201), lao4 (0), la4 (0)\\ 
    葛 & 196 & ge3 (175), ge2 (21)\\
    \multirow{2}{*}{蒙} & \multirow{2}{*}{197} &\multirow{2}{*}{meng2 (102), meng3 (94),} \\ 
    \multirow{2}{*}{} & \multirow{2}{*}{} & \multirow{2}{*}{meng1 (1)}\\
    {} & {} & {} \\
    蓼 & 202 & liao3 (202), lu4 (0)\\ 
    蔓 & 199 & man4 (182), man2 (17)\\ 
    蔚 & 192 & wei4 (151), yu4 (41)\\ 
    蕃 & 169 & bo1 (167), fan1 (2), fan2 (0)\\ 
    蕉 & 201 & jiao1 (201), qiao2 (0)\\ 
    薄 & 161 & bo2 (104), bao2 (51), bo4 (6)\\ 
    藉 & 196 & jie4 (150), ji2 (46)\\ 
    藏 & 199 & zang4 (131), cang2 (68)\\ 
    虾 & 201 & xia1 (200), ha2 (1)\\ 
    蚂 & 200 & ma3 (190), ma4 (9), ma1 (1)\\ 
    蚌 & 195 & beng4 (112), bang4 (83)\\ 
    蛤 & 200 & ge2 (198), ha2 (2)\\ 
    蜇 & 31 & zhe2 (22), zhe1 (9)\\ 
    蠡 & 179 & li3 (165), li2 (14)\\ 
    行 & 197 & xing2 (187), hang2 (10)\\ 
    衣 & 202 & yi1 (202), yi4 (0)\\ 
    衰 & 202 & shuai1 (200), cui1 (2)\\ 
    裨 & 141 & pi2 (118), bi4 (23)\\ 
    褚 & 200 & chu3 (199), zhu3 (1)\\ 
    褪 & 98 & tui4 (94), tun4 (4)\\ 
    褶 & 202 & zhe3 (202), xi2 (0)\\ 
    要 & 200 & yao4 (186), yao1 (14)\\ 
    覃 & 191 & tan2 (103), qin2 (88)\\ 
    见 & 199 & jian4 (199), xian4 (0)\\ 
    观 & 189 & guan1 (184), guan4 (5)\\ 
    觉 & 200 & jue2 (197), jiao4 (3)\\ 
    角 & 194 & jiao3 (113), jue2 (81)\\ 
    觜 & 12 & zi1 (12), zui3 (0)\\ 
    解 & 198 & jie3 (197), jie4 (1), xie4 (0)\\ 
    訾 & 19 & zi1 (18), zi3 (1)\\ 
    论 & 202 & lun4 (202), lun2 (0)\\ 
    识 & 200 & shi2 (200), zhi4 (0)\\ 
    语 & 202 & yu3 (202), yu4 (0)\\ 
    说 & 199 & shuo1 (198), shui4 (1)\\ 
    读 & 201 & du2 (201), dou4 (0)\\ 
    调 & 188 & diao4 (136), tiao2 (52)\\ 
    谜 & 201 & mi2 (201), mei4 (0)\\ 
    谥 & 202 & shi4 (202), yi4 (0)\\ 
    谩 & 50 & man4 (50), man2 (0)\\ 
    谯 & 200 & qiao2 (200), qiao4 (0)\\ 
    豁 & 175 & huo4 (126), huo1 (49), hua2 (0)\\ 
    豊 & 21 & li3 (20), feng1 (1)\\ 
    貉 & 13 & mo4 (13), he2 (0)\\ 
    贲 & 193 & ben1 (193), bi4 (0)\\ 
    贾 & 202 & jia3 (191), gu3 (11)\\ 
    赚 & 193 & zhuan4 (192), zuan4 (1)\\ 
    趟 & 201 & tang4 (199), tang1 (2)\\ 
    足 & 201 & zu2 (201), ju4 (0)\\ 
    \multirow{2}{*}{跂} & \multirow{2}{*}{12} &\multirow{2}{*}{qi3 (12), qi4 (0), zhi1 (0),} \\ 
    \multirow{2}{*}{} & \multirow{2}{*}{} & \multirow{2}{*}{ji1 (0), qi2 (0)}\\
    {}& {}& {} \\
    跄 & 8 & qiang4 (7), qiang1 (1)\\ 
    跑 & 201 & pao3 (200), pao2 (1)\\ 
    踏 & 200 & ta4 (198), ta1 (2)\\ 
    蹶 & 48 & jue2 (48), jue3 (0)\\ 
    车 & 201 & che1 (200), ju1 (1)\\ 
    轧 & 175 & zha2 (131), ya4 (42), ga2 (2)\\
    \multirow{2}{*}{转} & \multirow{2}{*}{199} &\multirow{2}{*}{zhuan3 (164), zhuan4 (35),} \\ 
    \multirow{2}{*}{} & \multirow{2}{*}{} & \multirow{2}{*}{ zhuai3 (0)}\\
    {}& {}& {} \\
    轲 & 99 & ke1 (99), ke3 (0)\\ 
    轴 & 201 & zhou2 (200), zhou4 (1)\\ 
    载 & 62 & zai4 (53), zai3 (9)\\ 
    辙 & 151 & zhe2 (151), che4 (0)\\ 
    辟 & 200 & pi4 (158), bi4 (42)\\ 
    边 & 200 & bian1 (186), bian5 (14)\\ 
    过 & 200 & guo4 (180), guo5 (20)\\ 
    还 & 198 & hai2 (186), huan2 (12)\\ 
    远 & 201 & yuan3 (201), yuan4 (0)\\ 
    迤 & 101 & yi3 (84), yi2 (17)\\ 
    追 & 202 & zhui1 (202), dui1 (0)\\ 
    适 & 202 & shi4 (202), kuo4 (0)\\ 
    通 & 202 & tong1 (202), tong4 (0)\\ 
    逮 & 199 & dai4 (197), dai3 (2)\\ 
    \multirow{2}{*}{那} & \multirow{2}{*}{200} &\multirow{2}{*}{na4 (200), nuo2 (0),} \\ 
    \multirow{2}{*}{} & \multirow{2}{*}{} & \multirow{2}{*}{ na1 (0), na3 (0)}\\
    {} & {} & {} \\
    都 & 195 & dou1 (144), du1 (51)\\ 
    酊 & 31 & ding1 (22), ding3 (9)\\ 
    酢 & 51 & cu4 (46), zuo4 (5)\\ 
    采 & 202 & cai3 (202), cai4 (0)\\ 
    重 & 197 & zhong4 (124), chong2 (73)\\ 
    量 & 198 & liang4 (189), liang2 (9)\\ 
    鉄 & 12 & tie3 (12), zhi4 (0)\\ 
    钉 & 195 & ding1 (138), ding4 (57)\\ 
    钌 & 52 & liao3 (52), liao4 (0)\\ 
    钯 & 202 & ba3 (202), pa2 (0)\\ 
    钻 & 181 & zuan4 (142), zuan1 (39)\\ 
    钿 & 50 & dian4 (50), tian2 (0)\\ 
    铛 & 52 & dang1 (50), cheng1 (2)\\ 
    铣 & 149 & xian3 (106), xi3 (43)\\ 
    铤 & 19 & ting3 (18), ding4 (1)\\ 
    铫 & 11 & yao2 (11), diao4 (0)\\ 
    铺 & 197 & pu4 (100), pu1 (97)\\ 
    锔 & 18 & ju2 (18), ju1 (0)\\ 
    锯 & 201 & ju4 (201), ju1 (0)\\ 
    镐 & 197 & hao4 (186), gao3 (11)\\ 
    镝 & 52 & di1 (32), di2 (20)\\ 
    镡 & 11 & tan2 (11), xin2 (0)\\ 
    长 & 198 & zhang3 (119), chang2 (79)\\ 
    閤 & 47 & ge2 (47), he2 (0)\\ 
    间 & 198 & jian1 (198), jian4 (0)\\ 
    闷 & 198 & men4 (150), men1 (48)\\ 
    阆 & 199 & lang4 (187), lang2 (12)\\ 
    阇 & 197 & du1 (197), she2 (0)\\ 
    阏 & 44 & yan1 (42), e4 (2)\\ 
    阙 & 157 & que4 (120), que1 (37)\\ 
    阿 & 202 & a1 (202), e1 (0)\\ 
    陂 & 200 & bei1 (200), po1 (0)\\ 
    陆 & 202 & lu4 (202), liu4 (0)\\ 
    降 & 199 & jiang4 (154), xiang2 (45)\\ 
    隆 & 202 & long2 (202), long1 (0)\\ 
    隐 & 202 & yin3 (202), yin4 (0)\\ 
    隗 & 143 & wei3 (143), kui2 (0)\\ 
    隽 & 147 & jun4 (117), juan4 (30)\\ 
    难 & 193 & nan2 (121), nan4 (72)\\ 
    雀 & 202 & que4 (202), qiao1 (0)\\ 
    雨 & 201 & yu3 (201), yu4 (0)\\ 
    露 & 193 & lu4 (175), lou4 (18)\\ 
    靓 & 88 & liang4 (88), jing4 (0)\\ 
    靡 & 199 & mi3 (100), mi2 (99)\\ 
    页 & 202 & ye4 (202), xie2 (0)\\ 
    顷 & 202 & qing3 (202), qing1 (0)\\ 
    颉 & 76 & jie2 (39), xie2 (37)\\ 
    颏 & 20 & ke1 (19), ke2 (1)\\ 
    食 & 175 & shi2 (175), si4 (0)\\ 
    饮 & 202 & yin3 (195), yin4 (7)\\ 
    馏 & 201 & liu2 (201), liu4 (0)\\ 
    馕 & 12 & nang2 (12), nang3 (0)\\ 
    驮 & 94 & tuo2 (94), duo4 (0)\\ 
    骑 & 182 & qi2 (175), ji4 (7)\\ 
    鬲 & 49 & li4 (32), ge2 (17)\\ 
    鲜 & 202 & xian3 (153), xian1 (49)\\ 
    鸟 & 202 & niao3 (202), diao3 (0)\\ 
    鹄 & 50 & hu2 (50), gu3 (0)\\ 
    龈 & 101 & yin2 (101), ken3 (0)
\end{supertabular}
